# Supplementary material for: Corpus Distillation for Effective Fuzzing: A Comparative Evaluation
Source: arXiv:1905.13055 source file (2020-09-21)
Supplement: Supplementary file 1 [file appendix-moonlight.tex]

\section{\tool Approach and Implementation}\label{sec:Theory-Appendix}

\paragraph{Problem definition}

Recall that a given target has a finite set of edges between its constituent
basic blocks, and any given seed will cause a subset of these edges to be
traversed when the target is executed on that seed.  This seed's set of edges
is its \emph{coverage}, and the coverage of a corpus is the union of all that
set's coverages.

\tool applies dynamic programming to take a large coverage matrix and
recursively transform it through row and column eliminations into successively
smaller matrices while accumulating a minimum cover set \coverset.

What follows is the key theoretical ideas that support our
algorithm, along with relevant supporting proofs.
First, we define the following notation:

\begin{itemize}[noitemsep]
\item $S$ is the set of all \emph{seeds} in the full corpus;
\item $E$ is the set of all \emph{edges} executed by the target for each element in~$S$;
\item $N = \|S\|$ is the number of seeds in the full corpus;
\item $M = \|E\|$ is the number of edges in the target;
\item $s_i \in S$ is the $i$th seed under some ordering;
\item $e_j \in E$ is the $j$th edge under some ordering;
  % Commented out because it is never used in this section
  %
  % \item $a_{ij} = \mathbb{I}[\text{\emph{seed} $i$ uses \emph{basic block
  %   edge} $j$}]$ where $\mathbb{I}$ is the \emph{indicator} function.
  %   The indicator function evaluates to 1 if the argument is true and 0
  %   otherwise.
\item $A = \Bigl[ a_{ij}\Bigr]$ is the~$N \times M$ corpus \textbf{coverage
    matrix}; and
\item Let~$c_i$ be the \emph{weight} of seed~$s_i$---a value to be defined but
  often~1 or the \emph{file size} of the seed or its execution time.
  % Commented out because it is never used in this section
  %
  % \item Let $x_i = \mathbb{I}[s_i \text{in the computed solution} ] $ be the
  %   decision vector for seeds that describes a solution.
  %   Practically, an element in the decision vector with value 1 means that
  %   the associated seed is included in the final fuzzing corpus.
\item $a_{ij} = \mathbb{I}[\text{\emph{seed} $i$ uses \emph{edge} $j$}]$
  where~$\mathbb{I}$ is the \emph{indicator} function; and
\item $x_i = \mathbb{I}[\text{$s_i$ in the computed solution}]$ be the
  decision vector for seeds that describes a solution.
\end{itemize}

We formulate our problem as a WMSCP described as follows:

\paragraph*{Objective}
\begin{align*}
  \min \sum_{i=1}^N c_i x_i
\end{align*}

\paragraph*{Subject to}
\begin{align*}
  \sum_{i=1}^N a_{ij} x_i \geq 1 &, \, \forall \, j \in \{1,...,M\} \text{ and} \\
  x_i \in \{0, 1\} &, \, \forall \, i \in \{1,...,N\}
\end{align*}

Once again, the objective is to find $\mathit{minset}(A)$, the smallest weighted set of seeds that still covers all the columns (edges) in matrix~$A$.
The unweighted version of the problem (the MSCP, as defined in \cref{sec:FormalCorpusDistillation}) sets~$c_i = 1, \forall i=\{1,...,N\}$.
This simply finds the smallest set of rows (i.e., the number of seeds) that spans all of the columns.
In the following presentation we generally do not distinguish between the weighted and unweighted formulations except where the distinction is important to the computation.

\subsection{Matrix Operations}\label{sec:matrix-ops}

The corpus coverage matrix~$A$ is typically large and sparse.  For
example, the number of seeds~$N$ in the corpus can be of the order of~$10^5$
files, while the number of observed edges is of the order of~$10^6$.  Combined,
the coverage matrix is of the order of~$10^{11}$ elements.

Before presenting the dynamic programming formulation and solution to this
problem, we first define the \emph{operational primitives} that allow us to
transform the large original problem into smaller overlapping sub-problems.

We begin with the following definitions.

\begin{itemize}[noitemsep]
\item $\rho$ denotes a subset of rows~$S$ in~$A$;
\item $\kappa$ denotes a subset of columns~$E$ in~$A$;
\item $A' = A \setminus_{\mathrm{row}} \rho$ denotes the matrix~$A$ with
  the rows~$\rho$ removed.  We term this \emph{row elimination};
\item $A'= A \setminus_{\mathrm{col}} \kappa$ denotes the matrix~$A$ with
  the columns~$\kappa$ removed (we term this \emph{column elimination});
\item
  $\Delta(A, \rho, \kappa) = A \setminus_{\mathrm{row}} \rho
  \setminus_{\mathrm{col}} \kappa$, which is the matrix~$A$ with rows~$\rho$
  and columns~$\kappa$ eliminated (we term this a \emph{matrix reduction});
  and
\item $\mathit{minset}(A)$ is the \emph{size} of the minimum cover set of
  matrix~$A$.
\end{itemize}

We proceed with the working example in \cref{fig:WorkingExampleMain}.  In this
example, rows~$s_i$ represent seeds and~$e_i$ represent all possible edges.

\begin{figure}[h]
  \centering
  \setlength{\lineskip}{1.5ex}% increase spacing
  \begin{subfigure}[b]{0.6\linewidth}
    \centering
    \scalebox{0.5}{
      \begin{tikzpicture}
        \example[1]
      \end{tikzpicture}
    }
    \caption{Coverage matrix}\label{fig:WorkingExampleMain}
  \end{subfigure}
  \begin{subfigure}[b]{0.49\linewidth}
    \centering
    \scalebox{0.5}{
      \begin{tikzpicture}
        % Singularity
        \example[0]
        \block[green]{1}{6} \block[green]{2}{6} \block[green]{3}{6}
        \block[green]{4}{6} \block[green]{5}{6}
      \end{tikzpicture}
    }
    \caption{Singularity}\label{fig:SingularityMain}
  \end{subfigure}
  \begin{subfigure}[b]{0.49\linewidth}
    \centering
    \scalebox{0.5}{
      \begin{tikzpicture}
        % Exotic
        \example[0]
        \block[cyan]{1}{2} \block[cyan]{1}{3} \block[cyan]{1}{5}
        \block[cyan]{1}{7}
        \highlight{1}{3} %mark the exotic seed-block
      \end{tikzpicture}
    }
    \caption{Exotic row}\label{fig:ExoticMain}
  \end{subfigure}
  \begin{subfigure}[b]{0.49\linewidth}
    \centering
    \scalebox{0.5}{
      \begin{tikzpicture}
        % Row Domination
        \example[0]
        \block[red]{5}{1} \block[red]{5}{2} \block[red]{5}{4}
        \block[red]{5}{5}
        \block[red]{5}{7}
        \block[yellow]{2}{2} \block[yellow]{2}{7}
        \block[yellow]{3}{1} \block[yellow]{3}{4} \block[yellow]{3}{5}
        \block[yellow]{4}{2} \block[yellow]{4}{5} \block[yellow]{4}{7}
      \end{tikzpicture}
    }
    \caption{Row dominance}\label{fig:RowDominanceMain}
  \end{subfigure}
  \begin{subfigure}[b]{0.49\linewidth}
    \centering
    \scalebox{0.5}{
      \begin{tikzpicture}
        % Column Domination
        \example[0]
        \block[red]{1}{5} \block[red]{3}{5} \block[red]{4}{5}
        \block[red]{5}{5}
        \block[yellow]{3}{1} \block[yellow]{5}{1}
        \block[yellow]{1}{3}
        \block[yellow]{3}{4} \block[yellow]{5}{4}
      \end{tikzpicture}
    }
    \caption{Column dominance}\label{fig:ColumnDominanceMain}
  \end{subfigure}
  \caption{Coverage minimization examples.  Rows $s_i$ represent seeds;
    columns $e_i$ represent all possible edges.  In (a), gray elements indicate edges
    that are covered by a given seed, while white elements indicate those
    edges that are uncovered.}
\end{figure}

%%% Local Variables:
%%% mode: latex
%%% TeX-master: "moonlight"
%%% End:

\subsubsection{Singularities}\label{AppSingularities}

We define the term \emph{singularity} to describe the situation where a column or row sum is \emph{zero}.
Additionally, we define the following:
\begin{itemize}[noitemsep]
\item Let~$\kappa_\theta = \theta(A)$ be the set of all \emph{singular
    columns} of matrix~$A$; and
\item Let~$A' = A \setminus_{\mathrm{col}} \kappa_\theta$ be the matrix~$A$ with the column singularities removed.
\end{itemize}

\begin{lemma}
  The matrix~$A'= A \setminus_{\mathrm{col}} \kappa_\theta$ has the same
  minimum cover set as~$A$.  That is, $\mathit{minset}(A) = \mathit{minset}(A')$.
  \begin{proof}
    Let the set of columns of~$A'$ be~$\kappa'$ and the set of
    columns of~$A$ be~$\kappa$.  Therefore~$\kappa = \kappa' \bigcup \kappa_\theta$.
    However no row exists that covers any column in~$\kappa_\theta$ otherwise
    the column would not be singular.  So any minimum cover set of~$A$ does not
    cover columns~$\kappa_\theta$ and so~$\kappa_\theta$ is superfluous to the
    computation.  Therefore any minimum cover set of~$A$ must also be a
    minimum cover set of~$A'$.
  \end{proof}
\end{lemma}

Row sum singularities represent seeds that do not cover any code when parsed by
the target.  These seeds are rare in practice and can simply be ignored.  In
contrast, column singularities are very common.  Column singularities are an
artifact of tracing tools that identified \emph{all} edges in the target.

Consider \cref{fig:SingularityMain} from the working example.  Column~$e_6$
(shown in green) is a singular column.  We can eliminate this column to
produce a smaller matrix~$A'$ whose minimum cover set~\coverset is the same as
the original matrix~$A$.

\subsubsection{Exotic Rows}

An \emph{exotic row} is the unique row~$s^*$ in~$A$ that covers~$e^*$.  For
example, in \cref{fig:ExoticMain} the row~$s_1$ (shown in blue) is exotic because it is the
only row that covers column~$e_3$.  All seeds associated with exotic rows are by definition
a part of the final solution and will be included in the distilled
corpus.

\begin{lemma}
  An exotic row is a member of any minimum cover set.
  \begin{proof}
    Almost by definition.  Any minimum cover set of~$A$ must include rows that
    cover all the non-singular columns.  An exotic row \emph{uniquely} covers
    at least one exotic column in~$A$ which forces its selection as a member
    of a minimum cover set.
  \end{proof}
\end{lemma}

Now:

\begin{itemize}[noitemsep]
\item Let~$S_\chi$ be the set of all exotic rows in~$A$; and
\item Let~$A' = A \setminus_{\mathrm{row}} S_\chi$.
\end{itemize}

\begin{lemma}
  $\mathit{minset}(A) = \mathit{minset}(A') + \|S_\chi\|$
  \begin{proof}
    Let~$s_i$ be an exotic row in~$A$.  Therefore~$s_i \in S_\chi$ by
    definition.  For convenience, let~$x = \mathit{minset}(A)$
    and~$y = \mathit{minset}(A')$.  Therefore~$x = y + 1$ since~$s_i$ must be
    in the optimal cover set and~$A$ and~$A'$ differ by only one row:
    the exotic row~$s_i$.  By induction for all rows in~$S_\chi$ the lemma
    follows.
  \end{proof}
\end{lemma}

\subsubsection{Dominant Rows}

Row dominance captures the intuitive idea that some rows in~$A$ may be
a subset of a single row.  The larger row \emph{dominates} the smaller
\emph{submissive} row which is a subset of the \emph{dominator}.  A
dominant row may in turn be dominated.  Intuitively, all submissive
rows can be deleted from the coverage matrix~$A$.  However, this
operation is row weight sensitive.  If the submissive row has a larger
row weight than the dominator then it can be deleted, else it is left
alone because it may ultimately lead to a smaller weighted corpus.
We make this notion more precise as follows:

\begin{itemize}[noitemsep]
\item Let~$s_\alpha$ be a row that covers the set of columns~$\alpha \subseteq E$;
\item Let~$s_\beta$ be a row that covers the set of columns~$\beta \subseteq \alpha$;
\item We say that~$s_\alpha$ \emph{dominates}~$s_\beta$;
\item We say that~$s_\beta$ \emph{submits} to~$s_\alpha$;
\item If~$s_\alpha^*$ has no dominators then we call it a \emph{primal dominator};
\item Let~$w_\alpha^*$ be the \emph{weight} of~$s_\alpha^*$;
\item Let~$S_\lambda$ be the set of \emph{all} rows that are dominated by~$s_\alpha^*$
  \emph{and whose individual row weights are less than or equal
  to}~$s_\alpha^*$.  We say that~$S_\lambda$ is a \emph{submissive set}
  of rows; and
\item Let $A' = A \setminus_{\mathrm{row}} \, S_\lambda$ be the matrix with
  the submissive rows from~$A$ removed.
\end{itemize}

Continuing with the (unweighted) working example in
\cref{fig:RowDominanceMain} we identify row~$s_5$ as a dominant row
(shown in red) since it dominates rows~$\{s_2,s_3,s_4\}$ (shown in
yellow).  The three submissive rows can be deleted from the matrix.

In the case of \emph{unweighted} distillations, row dominance and submission
strictly captures the idea that submissive rows are a proper subset cover of a
dominant row.  In the \emph{weighted} case only rows that are a proper
subset of a dominator \emph{and have a larger weight} then the dominator can
be removed.  Submissive rows with a smaller weight could in principle be
combined with another row whose combined weight is less than the dominant row
and therefore should not be removed.

\begin{lemma}
  $\mathit{minset}(A') = \mathit{minset}(A)$
  \begin{proof}
    For convenience let~$x= \mathit{minset}(A)$
    and~$y = \mathit{minset}(A')$.  Since~$A$ contains the primal dominator
    row~$s_\alpha^*$ none of the submissive rows in~$S_\lambda$ can be in
    the weighted minimum cover set.  If they were we could remove them to make
    a smaller weighted cover set giving a contradiction.  Therefore~$x$ does
    not count the submissive rows.  Additionally,~$A'$ does not contain
    the submissive rows since they were eliminated.  Therefore~$y$ could not
    include a count of these rows.  All else is equal so the lemma follows.
  \end{proof}
\end{lemma}

Eliminating a submissive row set allows us to transform a larger matrix into a
smaller one.  It is a very effective dimensional reduction technique in
practice.  The fact that \emph{weighted} row eliminations do not remove as
many rows as the \emph{unweighted} case will explain why weighted minimum
cover sets are usually larger (i.e., have more seeds) than unweighted ones.

\subsubsection{Dominant Columns}

Column dominance is a similar idea to row dominance.  Here, some
columns in~$A$ may be a subset of a single column.  However, in this
operation the dominant column is deleted and the submissive columns
are left alone.  This is because any final solution by definition will
contain seeds that cover the submissive columns and by implication
they will also cover the dominant column.  The dominant column is
redundant and can be safely removed.

Continuing with the working example in \cref{fig:ColumnDominanceMain} we
identify column~$e_5$ (shown in red) as a dominant column since it dominates
columns~$E_\mu = \{e_1,e_3,e_4 \}$.  Column~$e_2$ is not dominated by~$e_5$ because of~$s_2$.

\begin{itemize}[noitemsep]
\item Let~$e_\alpha$ be a column that covers the set of rows~$\alpha \subseteq S$;
\item Let~$e_\beta$ be a column that covers the set of rows~$\beta \subseteq \alpha$;
\item We say that~$e_\alpha$ \emph{dominates}~$e_\beta$;
\item We say that~$e_\beta$ \emph{submits} to~$e_\alpha$;
\item Let~$E_\mu$ be the set of all columns dominated by column~$e_\alpha$; and
\item Let $A' = A \setminus_{\mathrm{col}} e_\alpha$.
\end{itemize}

\begin{lemma}
  $\mathit{minset}(A') = \mathit{minset}(A)$
  \begin{proof}
    The minimum cover set~$S^*(A)$ must contain seeds which cover all
    of~$S_\alpha$.  However any seed that covers a column in~$S_\alpha$ must
    also cover~$e_\alpha$ since~$e_\alpha$ is a dominant column.
    Therefore any minimum cover set of
    $A' = A \setminus_{\mathrm{col}} e_\alpha$ is also going to be a minimum
    cover set of~$A$ since the dominant column is redundant in this case.
  \end{proof}
\end{lemma}

\subsubsection{Contained Columns}

When choosing row~$s_i$ to add to our solution we can eliminate all
the columns that~$s_i$ covers.  We call this operation \emph{contained
  column eliminations}.  The columns can be safely deleted because
they will be covered by the seed associated with row~$s_i$.

\begin{itemize}[noitemsep]
\item Let~$S_i$ be all the columns in~$A$ that~$s_i$ covers;
\item Let $A' = A \setminus_{\mathrm{row}} s_i$; and
\item Let $A'' = A' \setminus_{\mathrm{col}} S_i$.
\end{itemize}

\begin{lemma}
  $\mathit{minset}(A) - \mathit{minset}(A'') \leq 1$
  \begin{proof}
    For convenience let~$x = \mathit{minset}(A)$ and~$y = \mathit{minset}(A')$.
    Now there are two cases: if the selected row elimination is an optimal
    elimination then~$x = y$.  If the selected row that was eliminated is
    \emph{not} a member of a minimum cover set then~$x = y + 1$.  When we remove
    the columns~$S_i$ we know that~$s_i$ covers
    them.  Therefore these columns are no longer needed in calculating the
    solution.  Therefore~$\mathit{minset}(A'') = \mathit{minset}(A') = y$.
    Therefore~$x - y \leq 1$ and the lemma follows.
  \end{proof}
\end{lemma}

\subsubsection{Heuristic Row Reduction}

The row and column eliminations described previously have been
\emph{optimal} in the sense that they guarantee an optimal solution
for a smaller transformed matrix can be used to construct an optimal
solution for the larger matrix.  However, there are times when all
optimal operations are exhausted and the algorithm must make a
\emph{heuristic choice} to select a row to add to \coverset.
Intuitively, a good heuristic is to select the row with the largest
$\mathit{rowsum}$, since this will trigger a large \emph{contained
  columns elimination}.  In the weighted case, we choose the row with
the largest $\mathit{rowsum}/\mathit{rowweight}$.  The expectation is
that optimal operations can be resumed on the smaller matrix.

\subsection{\tool Algorithm}

We now present the \tool algorithm.
Given our matrix operators (\cref{sec:matrix-ops}), we use a dynamic programming formulation of the problem to compute a sequence of operations to construct \coverset.
The strategy is to apply these operators until the final operation results in the Null matrix, at which point no further operations are possible.

The Bellman Equation is the necessary condition for optimality when using
dynamic programming.  We define the \emph{state} of the problem to be
specified by the coverage matrix~$A$.  The \emph{cost} of the state is defined
to be the cost of any matrix operation performed on~$A$ denoted by~$d_*(A,A')$ plus the cost of the subsequent state~$A'$.
We want to choose the optimal transformation for state~$A$.  Therefore,
we define the Bellman equation for the problem as:
\begin{equation}
\mathit{Cost}(A) = \underset{i \in \{Operators\}}{\min}
\begin{cases}
d_i(A,A') + \mathit{Cost}(A') & A \neq Z\\
0 & A = Z
\end{cases}
\end{equation}
where the indexation consists of the five unary operations previously
specified.  We also make clear that any transformation from~$A \rightarrow A'$
implicitly uses the matrix reduction operation~$\Delta(\cdot)$ imposed on any
associated contained columns~$\kappa = \Pi(\cdot)$.

What are the costs~$d_*$ for each matrix operation?  Recall that our
objective is to find an optimal \coverset if possible, or measure
divergence from optimality when necessary.  Thus, any optimal row or
column elimination has zero cost because they contribute to an optimal~\coverset.
Optimal reductions occur when
$\mathit{minset}(A) = \mathit{minset}(A')\, \bigcup\, \textit{ExoticRow}$.  We
specify these reductions to have a zero cost \textit{iff} the matrix
size is reduced (i.e.,~$A \neq A'$); otherwise they have an infinite
cost.  For example, removing column singularities and selecting exotic
rows are all optimal operations and incur no cost providing they
reduce the size of the matrix~$A'$.  In contrast, heuristic row
reductions cannot be guaranteed to be an optimal reduction.
Therefore, we define the dynamic programming cost of this operation to
be:
\begin{myinlinelist}
\item \emph{one} for unweighted set cover; or
\item $\mathit{rowweight}$ for weighted set cover
\end{myinlinelist}.

\subsubsection{\tool Pseudocode}
We present pseudocode for \tool in \cref{alg:Moonshine}.  The ordering
of the five basic matrix operations reflects the relative importance
of those operations in either dimensional reduction, selecting
necessary rows, or computational complexity.
%%Given that matrix operation costs are zero apart from heuristic choice, this formulation of the algorithm is a correct encoding of the Bellman Equation outlined in \cref{DP}.
Observe that the heuristic row choice (i.e., the non-optimal
operation) is the last-resort option.

\begin{algorithm}[h]
  \footnotesize
\begin{algorithmic} % [1]
\Function{\tool}{$A$, $X$}
    \If {$\mathit{isEmpty}(A)$}
		\State \Return $X$
	\EndIf
    \State \Comment {Singularities}
    \State $\mathit{Cols} \leftarrow \mathit{Singularities}(A)$
    \If {$\mathit{Cols} \neq \emptyset$}
        \State $A' \leftarrow \mathit{RemoveRowsCols}(A, \emptyset, \mathit{Cols})$
		\State \Return \Call{\tool}{$A'$, $X$}
	\EndIf
    \State \Comment {Exotic rows}
    \State $\mathit{Rows} \leftarrow \mathit{Exotic}(A)$
    \If { $\mathit{Rows} \neq \emptyset$}
        \State $\mathit{Cols} \leftarrow \mathit{ContainedCols}(A, \mathit{Rows})$
        \State $A' \leftarrow \mathit{RemoveRowsCols}(A, \mathit{Rows}, \mathit{Cols})$
		\State $ X' \leftarrow X \bigcup Rows$
		\State \Return \Call{\tool}{$A'$, $X'$}
	\EndIf
    \State \Comment {Dominant rows}
    \State $\mathit{Rows} \leftarrow \mathit{DominantRows}(A)$
    \If { $\mathit{Rows} \neq \emptyset$}
        \State $A' \leftarrow \mathit{RemoveRowsCols}(A, \mathit{Rows}, \emptyset)$
		\State \Return \Call{\tool}{$A', X$}
	\EndIf
    \State \Comment {Dominant columns}
    \State $\mathit{Cols} \leftarrow \mathit{DominantCols}(A)$
    \If { $\mathit{Cols} \neq \emptyset$}
        \State $A' \leftarrow \mathit{RemoveRowsCols}(A, \emptyset, \mathit{Cols})$
		\State \Return \Call{\tool}{$A'$, $X$}
	\EndIf
    \State \Comment {Heuristic rows}
    \State $\mathit{Rows} \leftarrow \mathit{Heuristic}(A)$
    \State $\mathit{Cols} \leftarrow \mathit{ContainedCols}(A, \mathit{Rows})$
    \State $A' \leftarrow \mathit{RemoveRowsCols}(A, \mathit{Rows}, \mathit{Cols})$
    \State $X'  \leftarrow X \bigcup \mathit{Rows}$
	\State \Return \Call{\tool}{$A'$, $X'$}
\EndFunction
\State \Comment{Entry point}
\State $\mathit{Solution} \leftarrow$ \Call{\tool}{$A$, $\emptyset$}
\end{algorithmic}
\caption{\tool}
\label{alg:Moonshine}
\end{algorithm}

\subsection{Implementation}\label{MoonLightImpl}

We implemented \tool as a standalone tool in~\SI{2000}{\lines} of C++.
\tool takes as input a directory containing
\begin{myinlinelist}
\item the seed files to distill; and
\item for each seed file, a compressed code coverage trace.
\end{myinlinelist}

Because the number of seeds can be quite large, we store code coverage
as a \emph{bit vector} to reduce both storage costs and memory costs
when computing~$\mathit{minset}(A)$.  We provide a tool,
\emph{\bvtool} (implemented in~\SI{160}{\lines} of Python), to
generate these bit vector traces.  It converts the output of \showmap
(a tool included with AFL to display the coverage trace of a
particular input) to our bit vector representation.  The output of
\showmap is also used by \cmin.

Both \tool and \bvtool are open-sourced and available at
\url{https://bit.ly/2WZVynP}.

%%% Local Variables:
%%% mode: latex
%%% TeX-master: "moonlight"
%%% End:
